# Supplementary material for: Details Make a Difference: Object State-Sensitive Neurorobotic Task Planning
Source: arXiv:2406.09988 source file (2024-10-16)
Supplement: Supplementary file 1 [file Appendix.tex]

\section{Appendix}

\subsection{objects}
apple", "half apple" "bananas", "sliced bananas" "orange",
sliced oranges" "bow", "bow with soup"

\subsection{Object Detection}

\subsubsection{YOLO}

\subsubsection{OWL-ViT}

\subsubsection{OWL-V2}

\subsubsection{GPT4-V}
\subsubsection{GRiT}

\begin{figure}
    \centering
    \begin{subfigure}[b]{\columnwidth}
    \includegraphics[width=1\columnwidth]{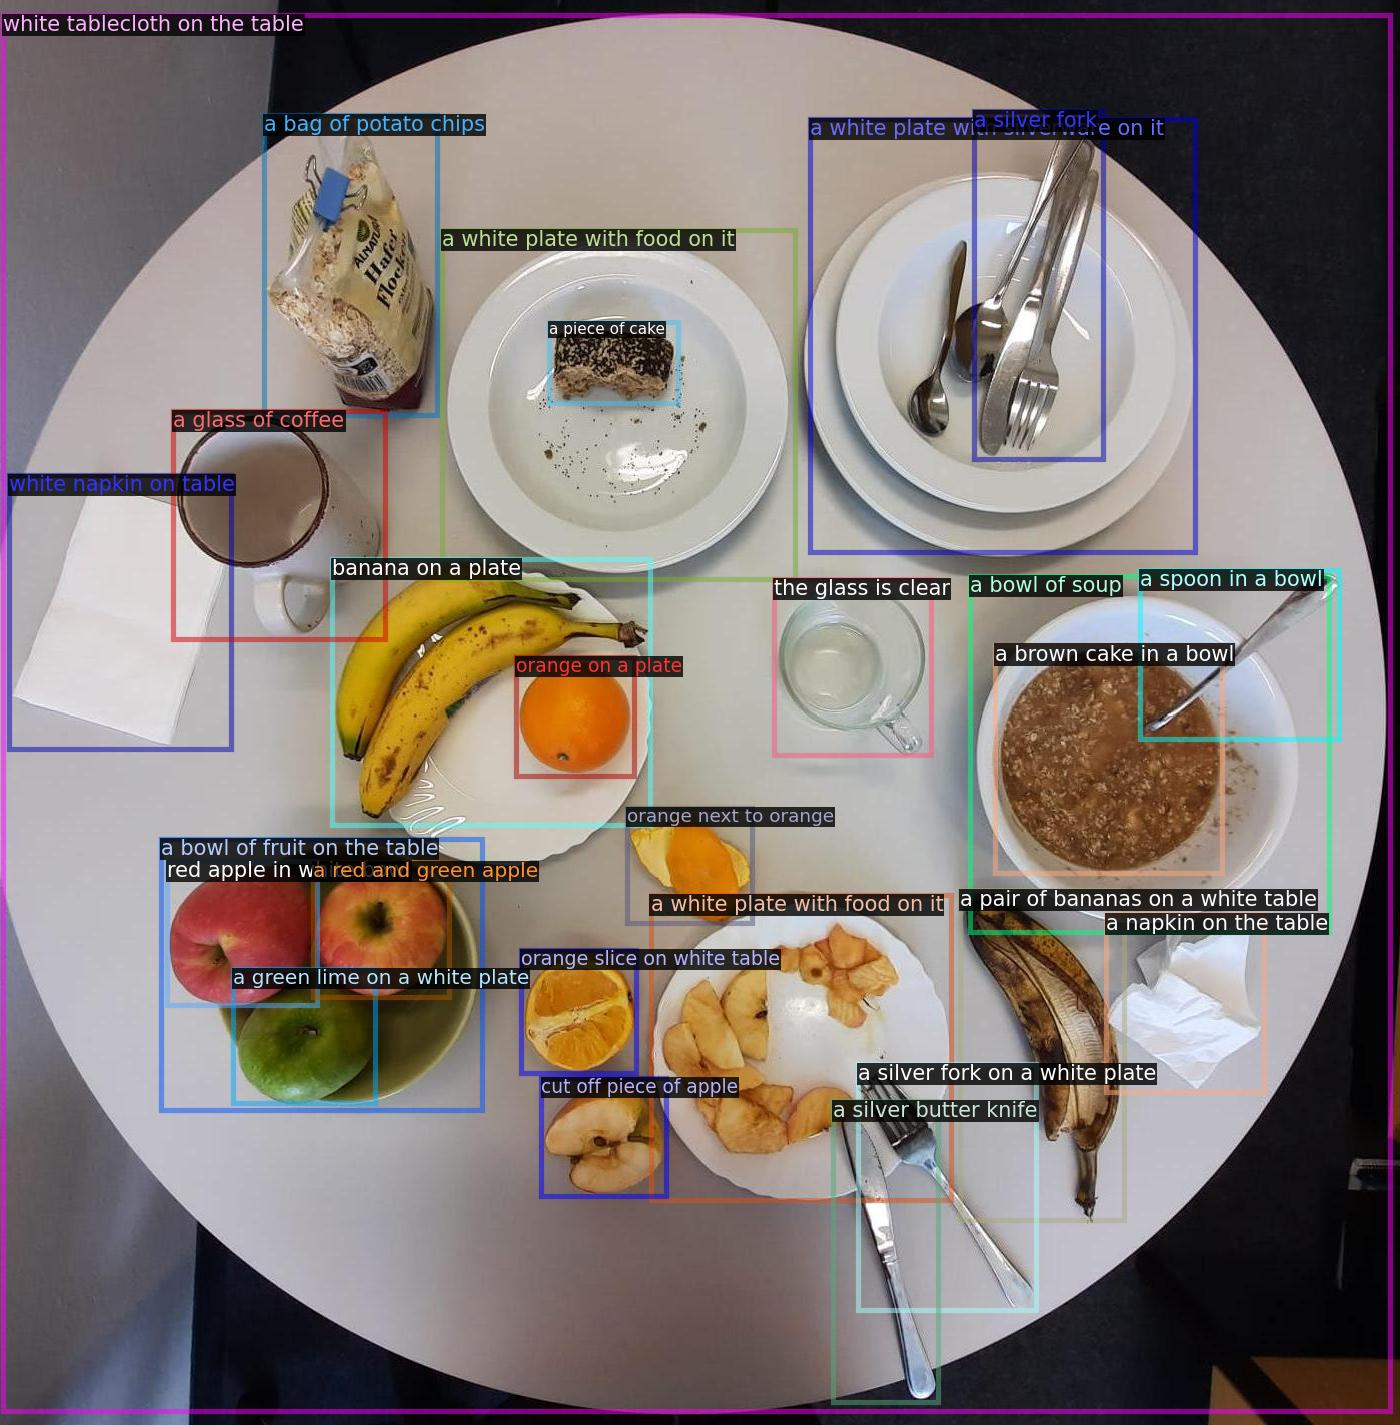}
    \vspace{-0.6cm}
    \caption{GRiT dense captioning.}
    \label{fig: method llm}
    \end{subfigure}
    %  \begin{subfigure}[b]{\columnwidth}
    % \includegraphics[width=1\columnwidth]{imgs/VLM.pdf}
    % \vspace{-0.6cm}
    % \caption{VLM-based Method.}
    % \label{fig: method vlm}
    % \end{subfigure}
    \caption{ The results of SOTA models.}
    \vspace{-0.6cm}
\end{figure}
\subsection{Annotation Format}
\begin{verbatim}
"object_name": {
    "color": "value1",
    "size": "value2",
    "shape": "value3",
    "container": true or false,
    "state": "value5",
    "destination": "value6",
    "grasping_type": "value7",
    "placing_type": "value8"
  }
\end{verbatim}
